# Supplementary material for: Probing Topological Floquet States in WSe$_2$ using Circular Dichroism in Time- and Angle-Resolved Photoemission Spectroscopy
Source: arXiv:2201.10476 source file (2022-01-25)
Supplement: Supplementary file 1 [file supplemental_note.pdf]

# Supplemental Note:
# Probing Topological Floquet States in $WSe_2$ using Circular Dichroism in Time- and Angle-Resolved Photoemission Spectroscopy

Michael Schüler[1] Samuel Beaulieu[2]

[1] *Condensed Matter Theory Group, Paul Scherrer Institute, CH-5232 Villigen PSI, Switzerland*

[2] *Université de Bordeaux - CNRS - CEA, CELIA, UMR5107, F33405, Talence, France*

## 1 Fitting the photoemission matrix elements

As explained in the methods section in the main text, the parameters defining the photoemission matrix elements are (i) two radial integrals for the Se-$p$ and the W-$d$ orbitals, respectively ($I^{(\pm)}_{p,d}$), (ii) the phase factors $\gamma_j$, and (iii) the inner potential $V_0$. The initial guesses for the parameters and the converged values are presented in Tab. 1. The radial integrals $I^{(\pm)}_{p,d}$ can be guessed from calculating them from the radial dependence of the Wannier orbitals, while the initial value for the inner potential is taken from ref. [1].

Table 1: Initial guesses for the fitting parameters and the optimized values.

| Parameter | Initial value | Final value |
|---|---|---|
| $I^{(-)}_p$ | -1.0 a.u. | -1.82688766 a.u. |
| $I^{(+)}_p$ | 0.8 a.u. | 2.845781 a.u. |
| $I^{(-)}_d$ | 0.02 a.u. | -0.03544242 a.u. |
| $I^{(-)}_d$ | 0.4 a.u. | -0.42897909 a.u. |
| $\gamma_1$ | 0 | -0.92774863 |
| $\gamma_2$ | 0 | 1.55128967 |
| $\gamma_3$ | 0 | 1.69446907 |
| $\gamma_4$ | 0 | 0.00771464 |
| $\gamma_5$ | 0 | -0.98096243 |
| $\gamma_6$ | 0 | 0.02939037 |
| $\gamma_7$ | 0 | -0.56628379 |
| $\gamma_8$ | 0 | -0.70343338 |
| $\gamma_9$ | 0 | 0.20267483 |
| $\gamma_1 0$ | 0 | 0.32908299 |
| $\gamma_1 1$ | 0 | 0.1826163 |
| $V_0$ | 0.175 a.u. | 0.137 a.u. |

As the objective of the minimization with add the squared differences of calculated and measured photoemission

intensity for $E - E_{\rm VBM} = -0.2$ eV close to all six valleys. The photoemission intensity is calculated from

$$I(\mathbf{k}, E) = |M_\alpha(\mathbf{k}, E)|^2 g(\varepsilon_\alpha(\mathbf{k}) + \omega_{\rm pr} - E) \ , \tag{1}$$

where $\alpha$ stands for top valence band and $g(\omega) = e^{-\omega^2/2\eta^2}/\sqrt{2\pi\eta^2}$ is a Gaussian function representing a broadened distribution. We fix $\eta = 0.0024$ a.u., matching the experimental resolution. The experimental spectra where shifted by 0.25 eV to match the EDC. The fitting is performed with a simulated annealing algorithm. The experimental data, the Wannier model and a script performing the fitting procedure are available at the repository schuel_m/fitting-matrix-elements at gitlab.psi.ch.

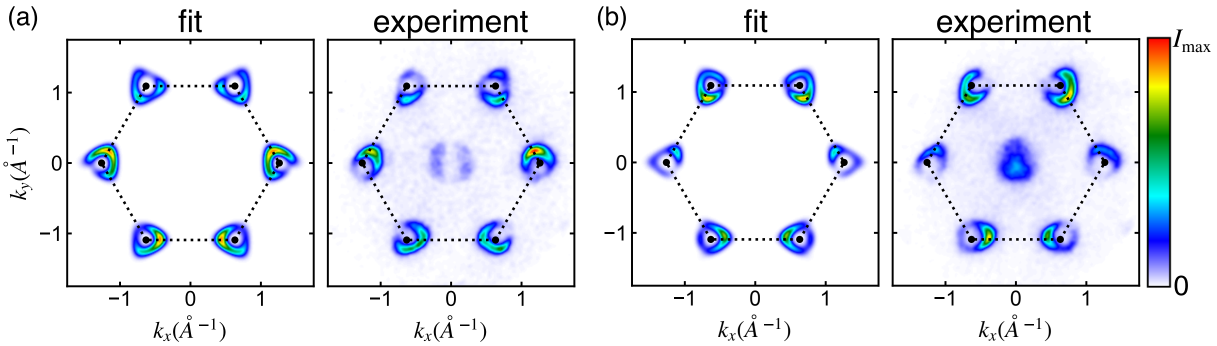


Figure 1: Comparison of the photoemission intensity calculated from Eq. (1) using optimized parameters in Tab. 1 and the experimental intensity for (a) $s$-polarized light, and (b) $p$-polarized photons.

## 2 Symmetry properties of the photoemission matrix elements

Let us assume that the Bloch state $|\psi_{\mathbf{k}\alpha}\rangle$ is composed only of the $d_{z^2}$ orbital localized at the W sites. In this case, the photoemission matrix elements with respect to $s$– and $p$–polarized light(dropping irrelavant phase factors) simplify to

$$M_s^{(2,0)}(\mathbf{k}, E) \propto \int d\mathbf{r}\, e^{-i\mathbf{p}\cdot\mathbf{r}} x \phi_{2,0}(\mathbf{r})$$
$$M_p^{(2,0)}(\mathbf{k}, E) \propto \int d\mathbf{r}\, e^{-i\mathbf{p}\cdot\mathbf{r}} (-y\cos\theta + z\sin\theta)\phi_{2,0}(\mathbf{r}) \ .$$

Here, $\phi_{2,0}(\mathbf{r}) = R(r)Y_{2,0}(\hat{\mathbf{r}})$, and the explicit expressions for the unit vectors $\mathbf{e}_{s,p}$ (see Fig. 1(b) in the main text) have been inserted. Now inverting the $k_x$ axis and using $\phi_{2,0}(\mathbf{r}) = \phi_{2,0}(-\mathbf{r})$ we find

$$M_p^{(2,0)}(-k_x, k_y, E) = M_p^{(2,0)}(k_x, k_y, E) \ , \quad M_s^{(2,0)}(-k_x, k_y, E) = -M_s^{(2,0)}(k_x, k_y, E) \ .$$

It is convenient to define the CDAD in terms of these matrix elements: $I_{\rm CD}(\mathbf{k}, E) \propto {\rm Im}[M_p^*(\mathbf{k}, E) M_s(\mathbf{k}, E)]$. Hence, for pure $d_{z^2}$ character, we find $I_{\rm CD}^{(2,0)}(-k_x, k_y, E) = -I_{\rm CD}^{(2,0)}(k_x, k_y, E)$.

For pure $d_{\pm 2}$ character of the Bloch state, the symmetry properties change as $\phi_{2,\pm 2}(-x, y, z) = \phi_{2,\mp 2}(x, y, z)$. Using these properties we find

$$M_p^{(2,\pm 2)}(-k_x, k_y, E) = M_p^{(2,\mp 2)}(k_x, k_y, E) \ , \quad M_s^{(2,\pm 2)}(-k_x, k_y, E) = -M_s^{(2,\mp 2)}(k_x, k_y, E)$$

and thus

$$I_{\rm CD}^{(2,\pm 2)}(-k_x, k_y, E) = -I_{\rm CD}^{(2,\mp 2)}(k_x, k_y, E) \approx I_{\rm CD}^{(2,\pm 2)}(k_x, k_y, E) \ .$$

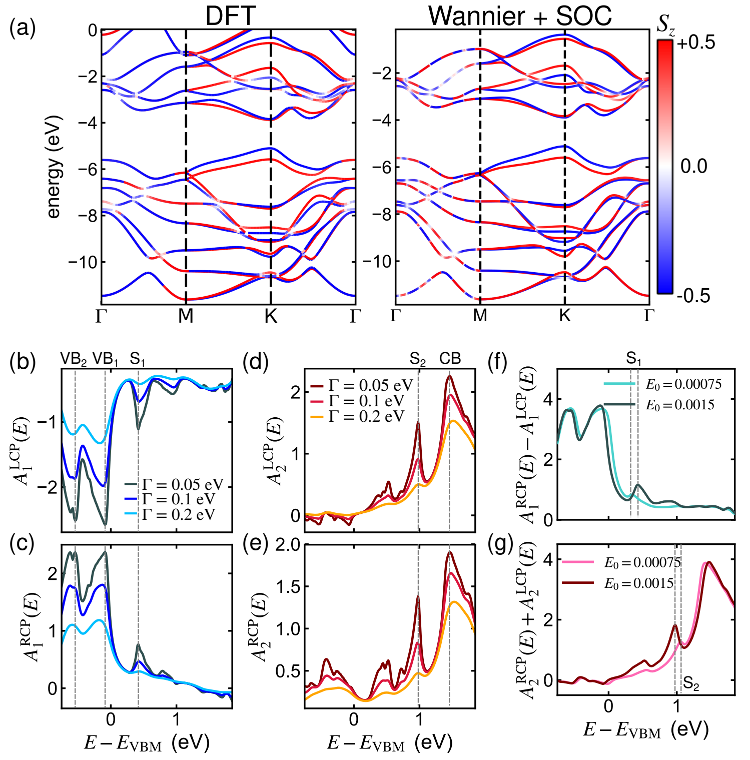


Figure 2: (a) Spin-resolved band structure and value of $S_z$ (represented by the color coding) of monolayer $WSe_2$ within (a) DFT calculations including SOC (otherwise identical to the nonrelativistic calculations discussed in the main text), and (b) within the Wannier model with $\lambda_{\mathrm{W}} = 0.13$ eV, $\lambda_{\mathrm{Se}} = 0.1$ eV. (b) Dichroic marker $A_1(E)$ for the orientation and LCP pump polarization as in Fig. 6(c) in the main text, and (c) for orientation and RCP pump polarization as in Fig. 6(c). (d), (e) dichroic marker $A_2(E)$ for crystal orientation as in (b), (c). The pump field strength is $E_0 = 1.5 \times 10^{-3}$ a.u. in (b)–(e), and the signal for different bath coupling strength $\Gamma$ is shown. The dashed lines indicate the first ($\mathrm{VB}_1$) and second ($\mathrm{VB}_2$) valence band, side band band ($S_{1,2}$), and conduction band (CB) peaks. (f) Time-reversal difference of the marker $A_1(E)$ for $\Gamma = 0.1$ eV for different field strength of the pump, and (g) marker $A_2(E)$.

The equality $I^{(2,\pm 2)}_{\mathrm{CD}}(k_x, k_y, E) = -I^{(2,\mp 2)}_{\mathrm{CD}}(k_x, k_y, E)$ holds for normal incidence. However, in a valley-averaged sense, we can treat the CDAD originating from $d_{+2}$ orbitals as qualitatively equal in each valley, and opposite upon the time-reversal operation $d_{+2} \leftrightarrow d_{-2}$.

# 3 Effects of spin-orbit coupling

We include spin-orbit coupling (SOC) into the Wannier Hamiltonian $H_{\alpha\alpha'}(\mathbf{k})$ (which has been constructed without SOC) by assuming atomic SOC:

$$H^{\mathrm{SOC}}_{\alpha\alpha'}(\mathbf{k}) = H_{\alpha\alpha'}(\mathbf{k}) + \sum_s \sum_{jj'} \lambda_s V^*_{j\alpha}(\mathbf{k}) [\mathbf{L}]^s_{jj'} \cdot \mathbf{S} V_{j'\alpha'}(\mathbf{k}) \, . \tag{2}$$

Here, $s \in \{\mathrm{W}, \mathrm{Se}\}$ runs over the atom types, $\mathbf{L}]^s_{jj'}$ is the matrix representation of the angular momentum operator with angular momentum $\ell = 1$ ($\ell = 2$) for $s = \mathrm{Se}$ ($s = \mathrm{W}$), and $V_{j\alpha}(\mathbf{k})$ are the eigenvectors of $H_{\alpha\alpha'}(\mathbf{k})$. $\mathbf{S}$ is the

spin operator. There are two parameters $\lambda_{\mathrm{Se,W}}$ that we fix such that the spin-resolved band structure matches the first-principle bands close to K and K′. The comparison is shown in Fig. 2(a).

Based on the Hamiltonian (2) we computed the pump-probe spin-integrated photoemission spectra in an analogous way as presented in the main text. Since band gap is reduced due to the SOC splitting, we chose $\hbar\omega_{\mathrm{p}} = 1.05$ eV to realize the same sub-gap pumping scenario and scaled the field strength accordingly. We show the dichroic markers as in Fig. 6 in the main text in Fig. 2(b)–(g). Apart from the spin-splitting of the valence band into $\mathrm{VB}_1$ and $\mathrm{VB}_2$ visible in Fig. 2(b), (c), and (f), the dichroic markers behave qualitatively the same as without SOC.

# References


[1] A. Rawat, N. Jena, Dimple, and A. De Sarkar, J. Mater. Chem. A **6**, 8693 (2018).
